# Supplementary material for: Private Hierarchical Clustering and Efficient Approximation
Source: arXiv:1904.04475 source file (2021-10-01)
Supplement: Supplementary file 2 [file appendix_subs.tex]

\section{Garbled circuits}
\label{sec:gc}

Here, we provide a more detailed description of garbled circuits and a running example in Figure~\ref{fig:garbled_circuit}.
We defer readers to~\cite{GC1,GC2} for a thorough formal treatment.
Consider two parties, $P_1$ and $P_2$
that wish to evaluate a function $f$ over their respective inputs $x_1,x_2$. One of the parties will play the role of the \emph{garbler} and the other will play the role of the \emph{evaluator}. Without loss of generality assume $P_1$ is the garbler and $P_2$ is the evaluator. Their interaction proceeds as follows.

\begin{figure}[tbph!]
	\includegraphics[width=.8\linewidth]{gc.pdf}
	\caption{Garbled circuit for a function that takes two bits from each party, computes their pairwise AND and an OR over the result.}\label{fig:garbled_circuit}
	\vspace{-0.3cm}
\end{figure}

%To better illustrate the concept of a garbled circuit

First $P_1$ expresses $f$ as a Boolean
circuit, i.e., as a directed acyclic graph of Boolean AND and OR gates,
and sends a ``garbled'' version of the circuit to $P_2$. We provide a concrete example in Figure~\ref{fig:garbled_circuit}
that depicts a Boolean circuit of two AND
gates $A,B$ and an OR gate $C$. The input $x_1$ is $11$ whereas $x_2$ is $01$ (both expressed in bits). The normal circuit should first compute the bitwise AND of the two
inputs and forwards the results to the OR gate. In order to garble the circuit, $P_1$ will pick two random values from a large domain (e.g., 128-bits each) for the two possible bits
of each wire of the circuit. We call  these the \emph{garbled values} for that wire.
More concretely, if the first (second) bit of $P_1$'s and $P_2$'s inputs
is to be inserted into gate $A$ (resp. $B$), $P_1$ selects $w_{11}^0, w_{11}^1,
w_{21}^0, w_{21}^1$ (resp. $w_{12}^0, w_{12}^1, w_{22}^0, w_{22}^1$). Mnemonically,
the subscript of a $w$ value for input wires corresponds to the party that provides it and the index of the bit on its input,
whereas the superscript indicates the wire's plaintext bit (e.g., $w_{21}^0$ is the value for $P_2$'s first bit in case that is a zero).
Proceeding further into the circuit,
$P_1$ picks $w_{A}^0, w_{A}^1, w_{B}^0, w_{B}^1,w_{C}^0, w_{C}^1$ for the possible bit outputs of
gates $A$, $B$, and $C$ respectively.
Without knowing how these random values where chosen, it is impossible to infer which corresponds to which bit.
Note that $w_{C}^0, w_{C}^1$ correspond to the final circuit output, i.e., to the value $f(x_1,x_2)$.

Next, $P_1$ creates a garbled truth table for every gate, which can be viewed as an encrypted version of the truth table of the Boolean gate. We explain this
only for gate $A$ and the other gates follow in a similar manner. The row
$(1,1) \rightarrow 1$ of the truth table of the AND gate $A$, should output $1$ on input
$1,1$. These inputs correspond to values $w_{11}^1, w_{21}^1$,
respectively, whereas the output corresponds to $w_{A}^1$. Using $w_{11}^1,
w_{21}^1$ as encryption keys in a symmetric encryption
scheme (e.g., 128-bit AES) $P_1$ \emph{double-encrypts} (i.e., encrypts twice in a layer manner) this possible output for $A$ as
$E_{w_{11}^1}(E_{w_{21}^1}(w_{A}^1))$. $P_1$ produces a
similar encryption for every row of the truth table of gate $A$ (and all other gates of the circuit) and sends them
to $P_2$, \emph{permuted} to hide the order of the rows. Observe that one can retrieve $w_{A}^1$
if and only if they possess \emph{both} $w_{11}^1, w_{21}^1$. Conversely, if one possesses
\emph{only} $w_{11}^1, w_{21}^1$, all other entries of the garbled truth table (besides $w_{A}^1$)
are indistinguishable from random, due to the semantic security of the encryption scheme.
In order for $P_2$ to be able to retrieve the final output, $P_1$ also sends the
output wire values $w_C^0,w_C^1$ \emph{together} with their corresponding mapping to 0 and 1.

%\begin{figure}[!t]
%	\centering
%	\includegraphics[width=0.6\linewidth]{Figures/garbled_circuit.eps}
%	%\vspace{-.8cm}
%	\caption{A garbled circuit example}
%	\label{fig:garbled_circuit}
%	%\ifeprint\else\vspace{-.5cm}\fi
%\end{figure}

Observe that, given the garbled truth tables values, if $P_2$ knows the $w$ value of each input wire of a
gate, she can easily discover its output value. For example, if she has
$w_{11}^1, w_{21}^1$, she can try to decrypt every value in the truth table until she
finds the correct value $w_{A}^1$.\footnote{\scriptsize For this, we need to assume that the encryption scheme allows
detection of well-formed decryptions, i.e., it is possible to deduce whether the retrieved plaintext has a correct format. This can be easily achieved using a blockcipher and padding with a sufficient number of $0$'s, in which case well-formed decryptions will have a long suffix of $0$'s and decryptions under the wrong key will have a suffix of random bits. This property is referred to as \emph{verifiable range} in~\cite{GC1}.} $P_2$ sends the
 $w$ values corresponding to his inputs ($w_{11}^1, w_{12}^0$) in the clear.
Since these are random values, $P_2$ cannot map them to 0 or 1, thus $P_1$'s input
is protected. The last technical challenge is for $P_2$ to retrieve the $w$ values corresponding
to \emph{his own} input (i.e., $w_{21}^1, w_{22}^1$), without telling $P_1$
which values he needs. (Recall that if $P_1$ just sends all of $w_{21}^0, w_{21}^1,w_{22}^1, w_{22}^0$, this allows more than one entries of the garbled truth table to be decrypted). This is achieved through a two-party secure computation protocol called
(1-out-of-2) \emph{oblivious transfer} (OT)~\cite{Rabin81}. At a very high level, and
focusing on the first bit of $S$'s input,  $P_2$ can retrieve via OT from $P_1$
exactly one value from pair ($w_{21}^0$, $w_{21}^1$), without $P_1$ learning
which of the two. To transfer all the necessary $w$ values,  the parties must execute (in parallel) an
OT protocol for every bit of $P_2$'s input. After retrieving these $w$ values, $P_2$  evaluates the circuit on her own as described above, and sends the output
bit (1 in our example) to $P_1$.

%If $U_q$ does not wish $S$ (the evaluator) to learn
%the output, she can omit sending to $S$ the final output mapping,  and instead
%store it locally. This property is called \emph{obliviousness}~\cite{BHR12}.

%There exist practical implementations of garbled circuits with very efficient
%garbling and evaluation tools (e.g.,~\cite{BHKR13,SHSSK15}), as well as
%compilers for translating a program written in a high-level language directly
%into a Boolean circuit (e.g., \cite{Fairplay04,HKSSW10}).

%\begin{algorithm}[th!bp]
%	\caption{$\minselect$ protocol between $\Pone$ and $\Ptwo$.}\label{alg:matrix_clustering}
%	\dnote{Garbage; needs to be re-written}
%	\PoneInput{$D=\{\en{d_1}\dots\en{d_m}\}$, $\pk'$}
%	\PtwoInput{$\pk', \sk'$}
%	%  \Output{Clusters}
%	$\Pone$ randomly generates $\{r_1, \dots, r_m\}$,
%	computes $\en{d_i'} = \en{d_i + r_i} = \en{d_i}\cdot\en{r_i}$ for $i = 1\dots m$,
%	and sends $\en{d_1'} \dots \en{d_n'}$ to $\Ptwo$\;
%	
%	$\Ptwo$ decrypts each $\en{d_i'}$\;
%	
%	\dnote{TODO: Explain the Garbled Circuit construction in detail. Also, discuss special symbol $\bot$.}
%	$\Pone$ and $\Ptwo$ execute the secure two-party computation protocol
%	to compute the position of the minimum value and
%	$\Pone$ gets $\ell$ such that $\ell= \argmin\{d_1, \dots, d_m\}$\;
%	
%	$\Pone$ outputs the index $\ell$.
%	
%	
%\end{algorithm}

\section{Sub-protocols for secure comparison}
\label{app:comp}

Here we show circuits for $\mathsf{ArgminSelect},\minselect$, and $\maxselect$ as defined in Section~\ref{sec:main}. These circuits are garbled and evaluated as described in Section~\ref{sec:prelims} and called as sub-routines during our protocol from Section~\ref{sec:main}, We assume values of $\lambda$ bits, and blinding randomness of $\kappa$ bits, which makes the sum $\kappa+1$ bits long. The final output of the circuit is denoted by an arrow in the figures.

\begin{figure}
	\centering
	\includegraphics[width=.25\linewidth]{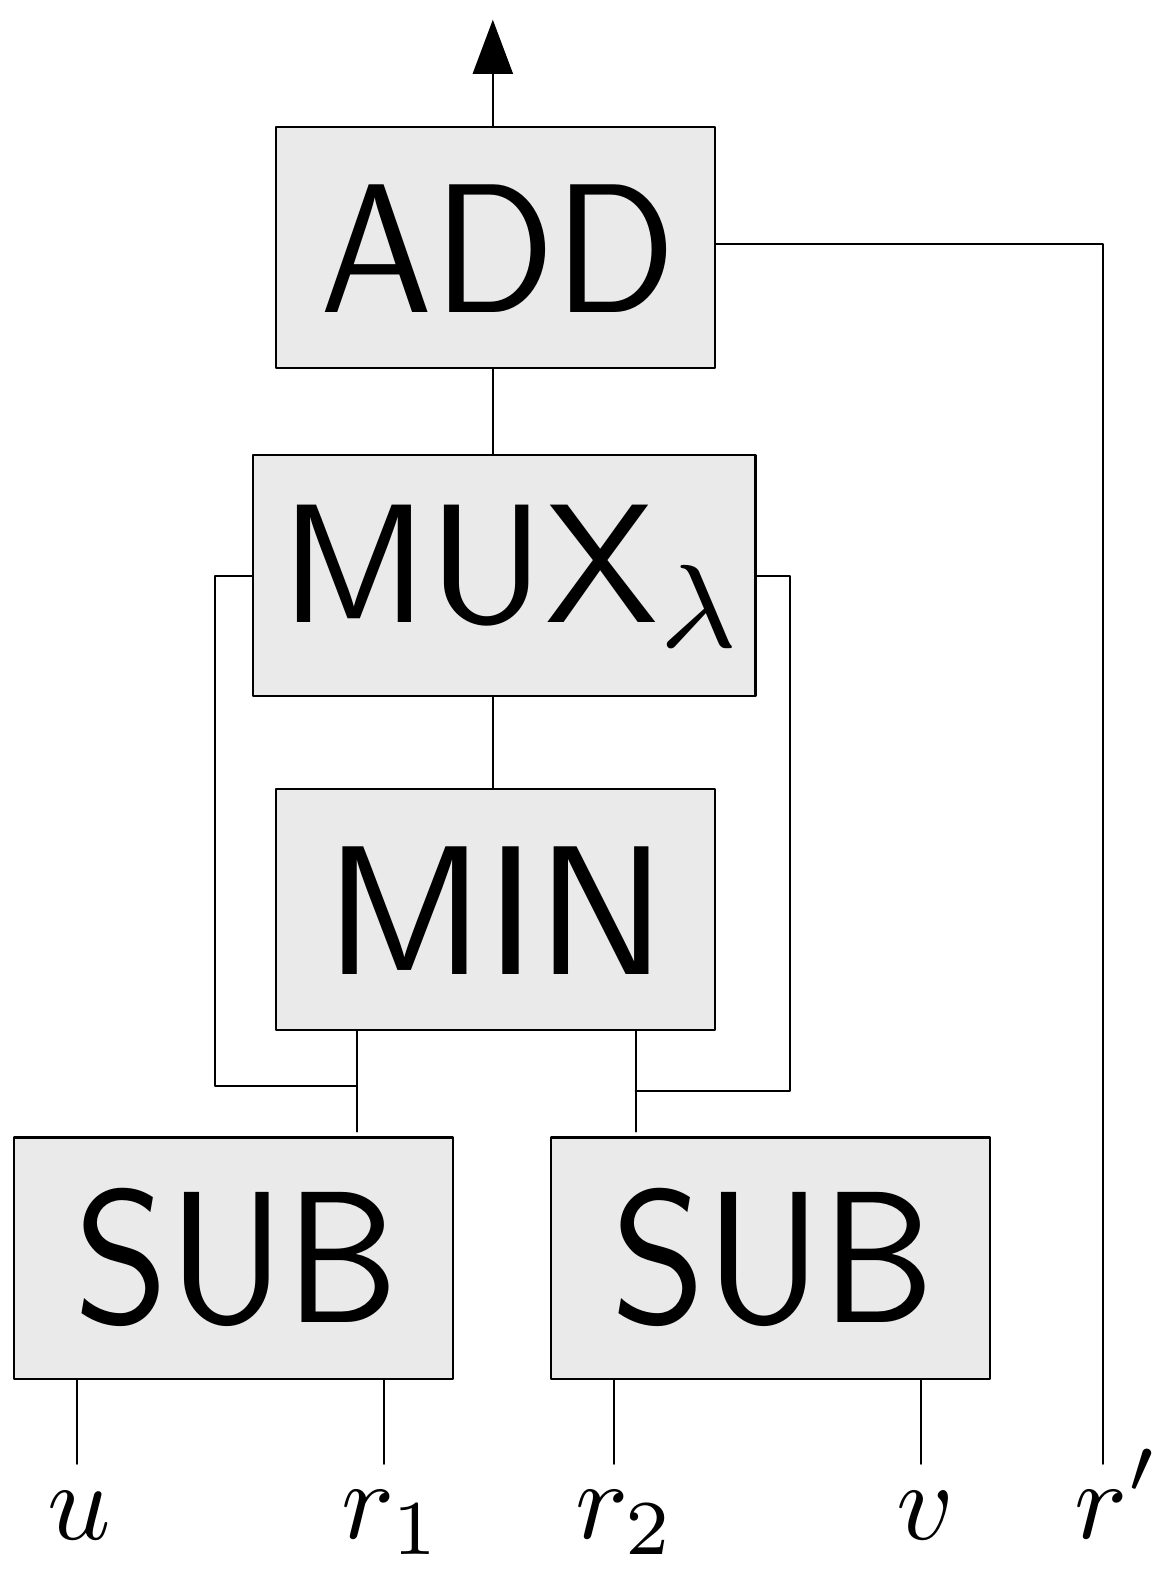}
	\caption{The circuit for $\minselect$.}\label{fig:sub1}
\end{figure}

The circuits use as building blocks gates for addition/subtraction \textsf{ADD}/\textsf{SUB} of $\kappa+1$-bit integers and minimum/maximum comparison \textsf{MIN}/\textsf{MAX} of two $\lambda$-bit integers. By convention, the latter output a single bit that indicates which is the minimum/maximum value (e.g., \textsf{MIN} on input $3,5$ outputs 0 to indicate the first value is smaller). We also need a multiplexer gate \textsf{MUX}$_i$ that upon input two inputs consisting of $i$ bits each, and a selector bit $s$ chooses the first or the second one, depending on the value of $s$.  The circuit for $\mathsf{ArgminSelect}$ operates on $n$ different inputs and  returns the index of the minimum one. To facilitate the final return of the index (without having to explicitly provide it as input), we hard-code in the circuit ``constant'' gates \textsf{CON}$_i$ that always output a fixed value $1\leq i \leq n$, e.g., \textsf{CON}$_3$ always outputs the binary representation of $3$ using $\log n$ bits. Alternatively, we could provide the indexes as input and ``carry'' them throughout the circuit. Efficient implementations for the above types of gates can be found in existing literature (e.g.,~\cite{min1}).

\begin{figure}
	\centering
	\includegraphics[width=.7\linewidth]{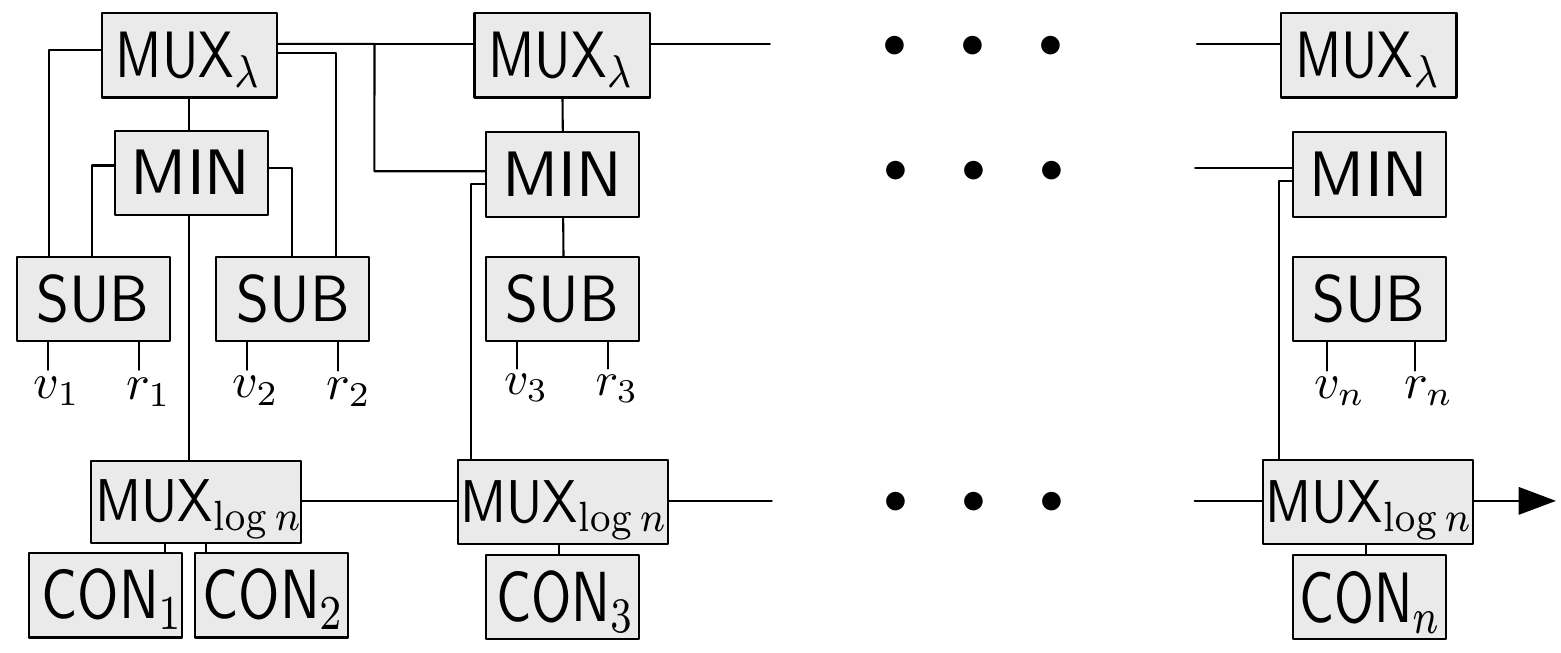}
	\caption{The circuit for $\mathsf{ArgminSelect}$.}\label{fig:sub2}
\end{figure}

Figure~\ref{fig:sub1} shows the circuit for $\minselect$. It takes as input five values $u,v,r_1,r_2,r'$ where the first two are of $\kappa+1$ bits and the last three are of $\kappa$ bits. It first computes $u-r_1$ and $v-r_2$ using two \textsf{SUB} gates. Then it computes the minimum of the two values using a \textsf{MIN} gate the output of which is forwarded to a \textsf{MUX}$_{\lambda}$ gate that takes as input the values $u-r_1$ and $v-r_2$. Finally, it blinds the output of the multiplexer again by adding $r'$ with a \textsf{ADD} gate, before outputting it. The circuit for $\maxselect$ is the same but uses a \textsf{MAX} gate instead.

Figure~\ref{fig:sub2} shows the circuit for $\mathsf{ArgminSelect}$. It takes as input $2n$ values $v_1,\dots,v_n$ and $r_1,\dots,r_n$. The first $n$ values are of $\kappa+1$ bits whereas the rest are of $\kappa$ bits. First, it uses $n$ \textsf{SUB} gates to compute values $v_i - r_i$ for $i=1,\dots,n$. Then it uses $n-1$ \textsf{MIN} gates to compare the minimum as follows. The first gate compares $v_1,v_2$. It outputs a bit that is fed to a  \textsf{MUX} gate as the selector. The input values for this multiplexer are provided by constant gates \textsf{CON}$_1$,\textsf{CON}$_2$. The output of \textsf{MIN} is also fed to another \textsf{MUX} gate that takes as input $v_1 - r_1$ and $v_2 - r_2$. The  outputs of the two multiplexer gates correspond to the current minimum value and index. They are then forwarded to a new   \textsf{MIN} gate for comparison with $v_3 - r_3$ and the process continues iteratively. For the $i$-th comparison, the index \textsf{MUX} gate will take the current minimum index and the output of \textsf{CON}$_{i+1}$. The final output after $n-1$ comparisons is given by the last index \textsf{MUX} gate.

% each input consists of $\kappa+1+\log n$ bits (where we assume that $\log n$ is an integer). The first $\kappa+1$  bits encode the blinded input itself, whereas the last $\log n$ bits encode its index among the $n$ inputs. We also require a selection gate \textsf{SEL}$(i,j)$ that upon input $

%%% Local Variables:
%%% mode: latex
%%% TeX-master: "paper"
%%% End:
